# Supplementary material for: Deep k-NN for Noisy Labels
Source: arXiv:2004.12289 source file (2020-04-26)
Supplement: Supplementary file 1 [file Appendix.tex]

\section{Experiment Details}

\textbf{Robust Generative Classifier (RoG):} \citet{lee2019robust} induces a generative classifier on top of the hidden feature spaces of a model pre-trained on noisy data. They assume the hidden features are Gaussian-distributed and estimate its parameters using the minimum covariance determinant estimator.  We always use $I_{\text{max}} = 2$, and train the ensemble over $40$ epochs of the filtered validation data using Adam with learning rate $0.001$. $50\%$ of the validation data was always kept and $2\%$ of the dataset was used for validation except for smaller UCI datasets, where $10\%$ was used. For ResNet-20 we use the convolutional and identity blocks within the final resnet block as hidden layers for RoG and use all intermediate dense layers for all other architectures.

\section{Proofs}
\subsection{Supporting theoretical results}

The following bounds $r_k(x)$ uniformly in $x \in \mathcal{X}$.
\begin{lemma}[Lemma 2 of \cite{jiang2019non}] \label{rkbound}
The following holds with probability at least $1 - \delta/2$.
If

\begin{align*}
2^8 \cdot D \log^2(4/\delta) \cdot \log n \le k \le \frac{1}{2} \cdot \omega  \cdot p_{X,0}\cdot v_D \cdot r_0^D \cdot n,
\end{align*}
then
$\sup_{x \in \mathcal{X}} r_k(x) \le \left( \frac{2k}{\omega \cdot v_D \cdot n \cdot p_{X, 0}}\right)^{1/D}$, where $v_D$ is the volume of the unit ball in $\R^D$.
\end{lemma}

The next result bounds the number of distinct $k$-NN sets over $\mathcal{X}$.
\begin{lemma}[Lemma 3 of \cite{jiang2019non}] \label{knncount}
Let $M$ be the number of distinct $k$-NN sets over $\mathcal{X}$, that is, $M := |\{ N_k(x) : x \in \mathcal{X} \}|$. 
Then $M \le D\cdot n^D$.
\end{lemma}

\subsection{Minimum $k$-NN spread}

We propose a more notion of how spread out a set of points is than $S_2$ which will be used in the theoretical analysis. This will allow us to more precisely characterize how difficult a configuration of incorrectly labeled examples will be to work with in the $k$-NN context. For example, if such examples are spread out far apart, then there will be many correctly labeled examples nearby for the $k$-NN approach to identify the incorrectly labeled examples. On the other hand, if the corrupted examples are all close together, then it will be more difficult to identify them without many uncorrected examples in that region. To this end, we define the minimum $k$-NN spread:

\begin{definition}
[minimum $k$-NN spread]
\begin{align*}
    S_k(C) := \min_{x \in C} r_k(x, C),
\end{align*}
where $r_k(x, C)$ denotes the distance from $x$ to the $k$-th closest neighbor in $C$.
\end{definition}
Note that this definition is consistent with the earlier definition of $S_2$.

\subsection{Proof of Theorem~\ref{theo:fixed_delta}}

\begin{proof}[Proof of Theorem~\ref{theo:fixed_delta}]
Let $\tau, \gamma, \epsilon > 0$ be quantities that will be determined later.
Suppose that for some $x \in \mathcal{X}^\Delta$, we have $r_k(x) \le \tau$ and $S_{\lfloor (\frac{1}{2} - \gamma)\cdot k \rfloor} (C) \ge \tau$.
Then, at least $\frac{1}{2} + \gamma$ fraction of the points within $x$'s $k$-nearest neighbors are not in the corrupted set $C$. Let $A_x := N_k(x) \backslash C$, that is, the $k$-nearest neighbors of $x$ that are not in $C$. Then it is clear that $A_x$ is a $k_0$-nearest neighbor set of $x$ relative to $X \backslash C$ for some $k_0 \ge \lceil (\frac{1}{2} + \gamma) \cdot k \rceil$. We have that $A_x \subseteq \X^{\Delta} \oplus \tau$ where $A\oplus r := \{x \in \X : \inf_{a \in A} |x - a| \le r\}$. Let us consider without loss of generality that $\eta(x) \ge \frac{1}{2} + \Delta$ (call this set $\X^{\Delta,+}$). The case $\X^{\Delta,-} := \{x \in \X^\Delta : \eta(x) \le \frac{1}{2} - \Delta\}$ follows by symmetry. 
Thus, we have $\eta(x') \ge \frac{1}{2} + \Delta - C_\alpha \tau^{\alpha}$ for all $x' \in A_x$. By Hoeffding's inequality, we have
\begin{align*}
    &\P\left(\frac{1}{|A_x|}\sum_{x' \in A_x} y(x') < \frac{1}{2} + \Delta - C_\alpha \tau^{\alpha} - \epsilon\right) \\
    &\le \exp(-2\epsilon^2 \cdot k_0),
\end{align*}
where $y(x)$ is the label corresponding to sample $x$.
By Lemma~\ref{knncount}, we have that there are at most $D\cdot n^D$ such $k_0$-nearest neighbor sets across all $k_0$ in $X \backslash C$. That is, this is also a bound on the number of distinct $A_x$ for $x \in \X$. Therefore, if we set 
\begin{align*}
\epsilon = \sqrt{\frac{D\log n + \log(4D/\delta)}{(1 + 2\gamma)\cdot k}},
\end{align*}
then by union bound, we have that 
\begin{align*}
    & \P\left(\inf_{x \in \X^{\Delta, +}}\frac{1}{|A_x|}\sum_{x' \in A_x} y(x') < \frac{1}{2} + \Delta - C_\alpha \tau^{\alpha} - \epsilon\right)\\
    &\le \frac{\delta}{4}.
\end{align*}
and thus, with probability at least $1 - \delta/4$, we have that 
$\frac{1}{|A_x|}\sum_{x' \in A_x} y(x') \ge \frac{1}{2} + \Delta - C_\alpha \tau^{\alpha} - \epsilon$ {\it uniformly} over $x \in \X^{\Delta,+}$.
Similarly, with probability at least $1 - \delta/4$ we have that
$\frac{1}{|A_x|}\sum_{x' \in A_x} y(x') \le \frac{1}{2} - \Delta + C_\alpha \tau^{\alpha} + \epsilon$ {\it uniformly} over $x \in \X^{\Delta,-}$.

Hence, in order for $k$-nearest neighbor prediction to predict the Bayes-optimal label on $\X^\Delta$, it  suffices that
\begin{align*}
    k_0 \left(\frac{1}{2} + \Delta - C_\alpha \tau^\alpha - \epsilon \right) \ge \frac{k}{2}.
\end{align*}
Since $k_0 \ge (\frac{1}{2} + \gamma) \cdot k$, we have that the above holds if
\begin{align*}
    \Delta \ge C_\alpha \tau^\alpha + \epsilon + \frac{1 - 2\gamma}{2(1 + 2\gamma)}.
\end{align*}
We now choose the values of $\tau, \gamma, \epsilon$ to upper bound each of the terms on the R.H.S. by $\Delta/3$ so that the above holds.

We can bound the last term by $\Delta/3$ by setting:
\begin{align*}
    \gamma = \frac{1}{2}\cdot \frac{3 - 2\Delta}{3 + 2\Delta}.
\end{align*}
Next, taking
\begin{align*}
    k \ge \frac{3(3 + 2\Delta)}{2\Delta^2} \left( D\log n + \log(4D/\delta) \right),
\end{align*}
we have that $\epsilon \le \Delta/3$.
Now, by Lemma~\ref{rkbound}, we have that setting
\begin{align*}
    \tau = \left(\frac{2k}{\omega \cdot v_D \cdot n \cdot p_{X, 0}} \right)^{1/D}
\end{align*}
gives us that $r_k(x) \le \tau$ for all $x \in \X$ with probability at least $1 - \delta/2$.
It thus suffices to take
\begin{align*}
k \le \frac{1}{2} \left( \frac{\Delta}{3\cdot C_\alpha}\right)^{D/\alpha}\cdot \omega \cdot v_D\cdot p_{X, 0} \cdot n
\end{align*}
so that $C_\alpha\tau^\alpha \le \Delta/3$.
Now in order for $S_{\lfloor (\frac{1}{2} - \gamma)\cdot k \rfloor} (C) \ge \tau$, it suffices to have $S_2(C) \ge \tau$. This can be accomplished by having the following hold:
\begin{align*}
    k \le \frac{1}{2}\cdot S_2(C)^{D}\cdot \omega \cdot v_D\cdot p_{X, 0} \cdot n.
\end{align*}
Thus, there exists positive constants $K_l$ and $K_u$ depending only on $\mathcal{F}$ such that if
\begin{align*}
k &\geq K_u \cdot \frac{1}{\Delta^2} \cdot (\log^2(1/\delta) \cdot \log n)\\
k &\le K_u \cdot \min\{S_2(C)^D, \Delta^{D/\alpha} \} \cdot n,
\end{align*}
then the desired conditions hold.
\end{proof}

\subsection{Proof of Theorem~\ref{theo:rates_delta}}

\begin{proof}[Proof of Theorem~\ref{theo:rates_delta}]
The proof begins in the same way as the proof of Theorem~\ref{theo:fixed_delta}.
As before, let $\tau, \gamma, \epsilon > 0$ be quantities that will be determined later. Like before, we are reduced to showing
\begin{align*}
    \Delta \ge C_\alpha \tau^\alpha + \epsilon + \frac{1 - 2\gamma}{2(1 + 2\gamma)},
\end{align*}
as long as the conditions for Lemma~\ref{rkbound} and~\ref{knncount} hold and $S_2(x) \ge \tau$ and $r_k(x) \le \tau$ where we choose
\begin{align*}
    \epsilon &= \sqrt{\frac{D\log n + \log(4D/\delta)}{(1 + 2\gamma)\cdot k}},\\
    \gamma &= \frac{1}{2}\cdot \frac{3 - 2\Delta}{3 + 2\Delta},\\
    \tau &= \left(\frac{2k}{\omega \cdot v_D \cdot n \cdot p_{X, 0}} \right)^{1/D}.
\end{align*}
These conditions hold for some $K_u$ and $K_l$ depending on $\mathcal{F}$.
Then we are reduced to having
\begin{align*}
    \frac{2}{3} \Delta &\ge \sqrt{\frac{D\log n + \log(4D/\delta)}{(1 + 2\gamma)\cdot k}}\\
    &+ C_\alpha \left(\frac{2k}{\omega \cdot v_D \cdot n \cdot p_{X, 0}} \right)^{\alpha/D}.
\end{align*}
Since $\gamma \ge 0$, it suffices to have
\begin{align*}
    \frac{2}{3} \Delta &\ge \sqrt{\frac{D\log n + \log(4D/\delta)}{k}}\\
    &+ C_\alpha \left(\frac{2k}{\omega \cdot v_D \cdot n \cdot p_{X, 0}} \right)^{\alpha/D}.
\end{align*}
The desired form for $\Delta$ clearly follows for some choice of $K$ depending only on $D, \omega, p_{X, 0}, C_\alpha$, all of which depend only on $\mathcal{F}$.

Finally, we must ensure that $\lfloor(\frac{1}{2} - \gamma)\cdot k \rfloor \ge 2$ so that $S_{\lfloor (\frac{1}{2} - \gamma)\cdot k \rfloor} (C)  \ge S_2(x)$.
Given the expression for $\gamma$, it is equivalent to have $\lfloor \left(\frac{2\Delta}{3 + 2\Delta} \right)\cdot k \rfloor \ge 2$. It suffices to show that $k \ge \frac{3(3+2\Delta)}{2\Delta}$. Given the form of $\Delta$ in terms of $n$ and $k$, we see that it suffices to have that
\begin{align*}
    k\ge \frac{9}{2}\cdot K\cdot \left(\sqrt{\frac{\log n + \log(1/\delta)}{k}} + \left(\frac{k}{n}\right)^{\alpha/D} \right)^{-1} + 3,
\end{align*}
which holds when $k \ge K_0 \cdot n^{2\alpha/(2\alpha + D)}$ for some $K_0$ depending only on $\mathcal{F}$, as desired.
\end{proof}

\subsection{Proof of Theorem~\ref{theo:rates_margin}}

\begin{proof}[Proof of Theorem~\ref{theo:rates_margin}]
The first part follows from Theorem~\ref{theo:rates_delta}. For the second part, we have by Theorem~\ref{theo:rates_delta} that if $x \in \mathcal{X}^\Delta$, then the $k$-NN classifier and the Bayes-optimal classifier match with probability $1- \delta$ uniformly. Thus, we have
\begin{align*}
    R_X - R^* &\le \P(x \not \in \X^\Delta) (\E_\mathcal{F}[g_k(x) \neq y|x \not\in \X^\Delta]\\
    &- \E_\mathcal{F}[ g^*(x) \neq y| x \not\in \X^\Delta]) \\
    &\le C_\beta \cdot \Delta^\beta \cdot (\E_\mathcal{F}[g_k(x) \neq y|x \not\in \X^\Delta]\\
    &- \E_\mathcal{F}[ g^*(x) \neq y| x \not\in \X^\Delta])\\
    &\le C_\beta \cdot \Delta^\beta \cdot 2\Delta.
\end{align*}
The result follows immediately from Theorem~\ref{theo:rates_delta}.
\end{proof}

\section{Hard Flip Permutations}
For Fashion MNIST we hard flip by swapping the following classes: TSHIRT $\leftrightarrow$ SHIRT, TROUSER $\leftrightarrow$ DRESS, PULLOVER $\leftrightarrow$ COAT, SANDAL $\leftrightarrow$ BAG, SNEAKER $\leftrightarrow$ ANKLEBOOT. For CIFAR10 we swap the pairs: TRUCK $\leftrightarrow$ AUTOMOBILE, BIRD $\leftrightarrow$ AIRPLANE, DEER $\leftrightarrow$ HORSE, CAT $\leftrightarrow$ DOG, FROG $\leftrightarrow$ SHIP. For CIFAR100, we hard flip circularly (i.e. $\pi(i) = (i+1) \mod K)$ within each of the 20 superclasses. For all other datasets, we hard flip
circularly.

\section{Area-Under-Curve Table}
We provide the Area-Under-the-Curve tables for the case when clean auxiliary data is available. These were omitted from the main text due to space constraints.

\begin{table*}[h!]
\centering
\begin{tabular}{|rccccccll|}
\hline
\multicolumn{1}{|l}{} & \multicolumn{1}{l}{} & \multicolumn{1}{l}{} & \multicolumn{1}{l}{Flip} & \multicolumn{1}{l}{} & \multicolumn{1}{l}{} & \multicolumn{1}{l}{} &  &  \\ \hline
\multicolumn{1}{|c|}{Dataset} & \multicolumn{1}{c|}{\% Clean} & \multicolumn{1}{l|}{Forward} & \multicolumn{1}{l|}{Clean} & \multicolumn{1}{l|}{Distill} & \multicolumn{1}{l|}{GLC} & \multicolumn{1}{l|}{k-NN} & \multicolumn{1}{l|}{k-NN Classify} & Full \\ \hline
\multicolumn{1}{|r|}{} & \multicolumn{1}{c|}{5} & \multicolumn{1}{c|}{4.83} & \multicolumn{1}{c|}{3.16} & \multicolumn{1}{c|}{2.96} & \multicolumn{1}{c|}{2.35} & \multicolumn{1}{c|}{\textbf{2.1}} & \multicolumn{1}{l|}{2.52} & 2.92 \\
\multicolumn{1}{|r|}{Letters} & \multicolumn{1}{c|}{10} & \multicolumn{1}{c|}{4.45} & \multicolumn{1}{c|}{2.52} & \multicolumn{1}{c|}{2.12} & \multicolumn{1}{c|}{1.92} & \multicolumn{1}{c|}{\textbf{1.8}} & \multicolumn{1}{l|}{2.06} & 2.49 \\
\multicolumn{1}{|r|}{} & \multicolumn{1}{c|}{20} & \multicolumn{1}{c|}{3.85} & \multicolumn{1}{c|}{2.07} & \multicolumn{1}{c|}{1.78} & \multicolumn{1}{c|}{1.56} & \multicolumn{1}{c|}{1.58} & \multicolumn{1}{l|}{\textbf{1.42}} & 1.93 \\ \hline
\multicolumn{1}{|r|}{} & \multicolumn{1}{c|}{5} & \multicolumn{1}{c|}{7.91} & \multicolumn{1}{c|}{1.93} & \multicolumn{1}{c|}{3.21} & \multicolumn{1}{c|}{2.16} & \multicolumn{1}{c|}{\textbf{1.34}} & \multicolumn{1}{l|}{3.97} & 4.31 \\
\multicolumn{1}{|r|}{Phonemes} & \multicolumn{1}{c|}{10} & \multicolumn{1}{c|}{7.95} & \multicolumn{1}{c|}{1.54} & \multicolumn{1}{c|}{2.75} & \multicolumn{1}{c|}{1.69} & \multicolumn{1}{c|}{\textbf{1.22}} & \multicolumn{1}{l|}{3.64} & 3.96 \\
\multicolumn{1}{|r|}{} & \multicolumn{1}{c|}{20} & \multicolumn{1}{c|}{7.89} & \multicolumn{1}{c|}{1.34} & \multicolumn{1}{c|}{1.97} & \multicolumn{1}{c|}{1.35} & \multicolumn{1}{c|}{\textbf{1.16}} & \multicolumn{1}{l|}{2.87} & 3.28 \\ \hline
\multicolumn{1}{|r|}{} & \multicolumn{1}{c|}{5} & \multicolumn{1}{c|}{5.27} & \multicolumn{1}{c|}{0.56} & \multicolumn{1}{c|}{3.89} & \multicolumn{1}{c|}{0.53} & \multicolumn{1}{c|}{\textbf{0.52}} & \multicolumn{1}{l|}{5.15} & 4.95 \\
\multicolumn{1}{|r|}{Wilt} & \multicolumn{1}{c|}{10} & \multicolumn{1}{c|}{5.63} & \multicolumn{1}{c|}{0.44} & \multicolumn{1}{c|}{3.14} & \multicolumn{1}{c|}{0.43} & \multicolumn{1}{c|}{\textbf{0.41}} & \multicolumn{1}{l|}{4.86} & 4.84 \\
\multicolumn{1}{|r|}{} & \multicolumn{1}{c|}{20} & \multicolumn{1}{c|}{5.18} & \multicolumn{1}{c|}{0.34} & \multicolumn{1}{c|}{2.67} & \multicolumn{1}{c|}{0.35} & \multicolumn{1}{c|}{\textbf{0.34}} & \multicolumn{1}{l|}{4.23} & 4.32 \\ \hline
\multicolumn{1}{|r|}{} & \multicolumn{1}{c|}{5} & \multicolumn{1}{c|}{5.13} & \multicolumn{1}{c|}{4.33} & \multicolumn{1}{c|}{5.56} & \multicolumn{1}{c|}{4.39} & \multicolumn{1}{c|}{\textbf{3.64}} & \multicolumn{1}{l|}{5.11} & 4.88 \\
\multicolumn{1}{|r|}{Seeds} & \multicolumn{1}{c|}{10} & \multicolumn{1}{c|}{5.02} & \multicolumn{1}{c|}{3.38} & \multicolumn{1}{c|}{4.58} & \multicolumn{1}{c|}{3.19} & \multicolumn{1}{c|}{\textbf{2.65}} & \multicolumn{1}{l|}{4.9} & 4.73 \\
\multicolumn{1}{|r|}{} & \multicolumn{1}{c|}{20} & \multicolumn{1}{c|}{4.41} & \multicolumn{1}{c|}{2.56} & \multicolumn{1}{c|}{3.57} & \multicolumn{1}{c|}{2.65} & \multicolumn{1}{c|}{\textbf{2.09}} & \multicolumn{1}{l|}{4.23} & 3.86 \\ \hline
\multicolumn{1}{|r|}{} & \multicolumn{1}{c|}{5} & \multicolumn{1}{c|}{5.25} & \multicolumn{1}{c|}{3.38} & \multicolumn{1}{c|}{5.15} & \multicolumn{1}{c|}{4.03} & \multicolumn{1}{c|}{\textbf{3.02}} & \multicolumn{1}{l|}{4.32} & 4.43 \\
\multicolumn{1}{|r|}{Iris} & \multicolumn{1}{c|}{10} & \multicolumn{1}{c|}{5.06} & \multicolumn{1}{c|}{2.53} & \multicolumn{1}{c|}{4.58} & \multicolumn{1}{c|}{2.24} & \multicolumn{1}{c|}{\textbf{2.17}} & \multicolumn{1}{l|}{3.98} & 4.08 \\
\multicolumn{1}{|r|}{} & \multicolumn{1}{c|}{20} & \multicolumn{1}{c|}{4.46} & \multicolumn{1}{c|}{1.51} & \multicolumn{1}{c|}{3.45} & \multicolumn{1}{c|}{\textbf{1.38}} & \multicolumn{1}{c|}{1.46} & \multicolumn{1}{l|}{3.36} & 3.53 \\ \hline
\multicolumn{1}{|r|}{} & \multicolumn{1}{c|}{5} & \multicolumn{1}{c|}{5.17} & \multicolumn{1}{c|}{3.55} & \multicolumn{1}{c|}{4.49} & \multicolumn{1}{c|}{4.1} & \multicolumn{1}{c|}{\textbf{3.36}} & \multicolumn{1}{l|}{5.34} & 5.35 \\
\multicolumn{1}{|r|}{Parkinsons} & \multicolumn{1}{c|}{10} & \multicolumn{1}{c|}{5.43} & \multicolumn{1}{c|}{3.38} & \multicolumn{1}{c|}{4.25} & \multicolumn{1}{c|}{3.44} & \multicolumn{1}{c|}{\textbf{3.32}} & \multicolumn{1}{l|}{5.27} & 5.13 \\
\multicolumn{1}{|r|}{} & \multicolumn{1}{c|}{20} & \multicolumn{1}{c|}{5.19} & \multicolumn{1}{c|}{3.02} & \multicolumn{1}{c|}{3.94} & \multicolumn{1}{c|}{3.05} & \multicolumn{1}{c|}{\textbf{2.95}} & \multicolumn{1}{l|}{4.99} & 5.06 \\ \hline
\multicolumn{1}{|r|}{} & \multicolumn{1}{c|}{5} & \multicolumn{1}{c|}{3.6} & \multicolumn{1}{c|}{0.69} & \multicolumn{1}{c|}{1.91} & \multicolumn{1}{c|}{0.5} & \multicolumn{1}{c|}{\textbf{0.44}} & \multicolumn{1}{l|}{3.46} & 3.49 \\
\multicolumn{1}{|r|}{MNIST} & \multicolumn{1}{c|}{10} & \multicolumn{1}{c|}{3.22} & \multicolumn{1}{c|}{0.5} & \multicolumn{1}{c|}{1.5} & \multicolumn{1}{c|}{0.42} & \multicolumn{1}{c|}{\textbf{0.35}} & \multicolumn{1}{l|}{3.1} & 3.14 \\
\multicolumn{1}{|r|}{} & \multicolumn{1}{c|}{20} & \multicolumn{1}{c|}{2.48} & \multicolumn{1}{c|}{0.35} & \multicolumn{1}{c|}{0.86} & \multicolumn{1}{c|}{0.34} & \multicolumn{1}{c|}{\textbf{0.27}} & \multicolumn{1}{l|}{2.36} & 2.41 \\ \hline
\multicolumn{1}{|r|}{} & \multicolumn{1}{c|}{5} & \multicolumn{1}{c|}{3.55} & \multicolumn{1}{c|}{1.87} & \multicolumn{1}{c|}{2.55} & \multicolumn{1}{c|}{\textbf{1.59}} & \multicolumn{1}{c|}{1.6} & \multicolumn{1}{l|}{3.3} & 3.31 \\
\multicolumn{1}{|r|}{Fashion MNIST} & \multicolumn{1}{c|}{10} & \multicolumn{1}{c|}{3.14} & \multicolumn{1}{c|}{1.71} & \multicolumn{1}{c|}{2.13} & \multicolumn{1}{c|}{\textbf{1.53}} & \multicolumn{1}{c|}{1.54} & \multicolumn{1}{l|}{2.92} & 2.99 \\
\multicolumn{1}{|r|}{} & \multicolumn{1}{c|}{20} & \multicolumn{1}{c|}{2.38} & \multicolumn{1}{c|}{1.56} & \multicolumn{1}{c|}{1.54} & \multicolumn{1}{c|}{1.46} & \multicolumn{1}{c|}{\textbf{1.46}} & \multicolumn{1}{l|}{2.17} & 2.27 \\ \hline
\multicolumn{1}{|r|}{} & \multicolumn{1}{c|}{5} & \multicolumn{1}{c|}{7.14} & \multicolumn{1}{c|}{7.2} & \multicolumn{1}{c|}{7.12} & \multicolumn{1}{c|}{5.52} & \multicolumn{1}{c|}{\textbf{5.35}} & \multicolumn{1}{l|}{6.71} & 7.12 \\
\multicolumn{1}{|r|}{CIFAR10} & \multicolumn{1}{c|}{10} & \multicolumn{1}{c|}{6.82} & \multicolumn{1}{c|}{6.56} & \multicolumn{1}{c|}{6.72} & \multicolumn{1}{c|}{5.62} & \multicolumn{1}{c|}{\textbf{5.32}} & \multicolumn{1}{l|}{6.48} & 6.83 \\
\multicolumn{1}{|r|}{} & \multicolumn{1}{c|}{20} & \multicolumn{1}{c|}{6.62} & \multicolumn{1}{c|}{5.59} & \multicolumn{1}{c|}{5.9} & \multicolumn{1}{c|}{5.16} & \multicolumn{1}{c|}{\textbf{4.85}} & \multicolumn{1}{l|}{6.1} & 6.56 \\ \hline
\multicolumn{1}{|r|}{} & \multicolumn{1}{c|}{5} & \multicolumn{1}{c|}{10.79} & \multicolumn{1}{c|}{10.24} & \multicolumn{1}{c|}{10.03} & \multicolumn{1}{c|}{9.64} & \multicolumn{1}{c|}{9.66} & \multicolumn{1}{l|}{\textbf{9.2}} & 9.29 \\
\multicolumn{1}{|r|}{CIFAR100} & \multicolumn{1}{c|}{10} & \multicolumn{1}{c|}{10.81} & \multicolumn{1}{c|}{9.89} & \multicolumn{1}{c|}{9.68} & \multicolumn{1}{c|}{9.46} & \multicolumn{1}{c|}{9.63} & \multicolumn{1}{l|}{\textbf{9.1}} & 9.25 \\
\multicolumn{1}{|r|}{} & \multicolumn{1}{c|}{20} & \multicolumn{1}{c|}{10.8} & \multicolumn{1}{c|}{9.44} & \multicolumn{1}{c|}{9.13} & \multicolumn{1}{c|}{8.97} & \multicolumn{1}{c|}{9.17} & \multicolumn{1}{l|}{\textbf{8.92}} & 9.09 \\ \hline
\multicolumn{1}{|r|}{} & \multicolumn{1}{c|}{5} & \multicolumn{1}{c|}{5.6} & \multicolumn{1}{c|}{3.65} & \multicolumn{1}{c|}{4.09} & \multicolumn{1}{c|}{2.17} & \multicolumn{1}{c|}{\textbf{2.05}} & \multicolumn{1}{l|}{5.23} & 5.52 \\
\multicolumn{1}{|r|}{SVHN} & \multicolumn{1}{c|}{10} & \multicolumn{1}{c|}{5.5} & \multicolumn{1}{c|}{2.28} & \multicolumn{1}{c|}{3.72} & \multicolumn{1}{c|}{2.29} & \multicolumn{1}{c|}{\textbf{1.48}} & \multicolumn{1}{l|}{4.96} & 5.29 \\
\multicolumn{1}{|l|}{} & \multicolumn{1}{c|}{20} & \multicolumn{1}{c|}{4.85} & \multicolumn{1}{c|}{1.83} & \multicolumn{1}{c|}{3.09} & \multicolumn{1}{c|}{1.9} & \multicolumn{1}{c|}{\textbf{1.19}} & \multicolumn{1}{l|}{4.34} & 4.82 \\ \hline
\end{tabular}
\caption{AUC for Flip corruption type.}
\end{table*}

\begin{table*}[h!]
\centering
\begin{tabular}{|rccccccll|}
\hline
\multicolumn{1}{|l}{} & \multicolumn{1}{l}{} & \multicolumn{1}{l}{} & \multicolumn{1}{l}{Hard Flip} & \multicolumn{1}{l}{} & \multicolumn{1}{l}{} & \multicolumn{1}{l}{} &  &  \\ \hline
\multicolumn{1}{|c|}{Dataset} & \multicolumn{1}{l|}{\% Clean} & \multicolumn{1}{l|}{Forward} & \multicolumn{1}{l|}{Clean} & \multicolumn{1}{l|}{Distill} & \multicolumn{1}{l|}{GLC} & \multicolumn{1}{l|}{k-NN} & \multicolumn{1}{l|}{k-NN Classify} & Full \\ \hline
\multicolumn{1}{|r|}{} & \multicolumn{1}{c|}{5} & \multicolumn{1}{c|}{3.77} & \multicolumn{1}{c|}{3.17} & \multicolumn{1}{c|}{2.1} & \multicolumn{1}{c|}{1.83} & \multicolumn{1}{c|}{\textbf{1.82}} & \multicolumn{1}{l|}{1.82} & 2.52 \\
\multicolumn{1}{|r|}{Letters} & \multicolumn{1}{c|}{10} & \multicolumn{1}{c|}{3.63} & \multicolumn{1}{c|}{2.52} & \multicolumn{1}{c|}{1.85} & \multicolumn{1}{c|}{1.6} & \multicolumn{1}{c|}{\textbf{1.6}} & \multicolumn{1}{l|}{1.64} & 2.36 \\
\multicolumn{1}{|r|}{} & \multicolumn{1}{c|}{20} & \multicolumn{1}{c|}{3.35} & \multicolumn{1}{c|}{2.05} & \multicolumn{1}{c|}{1.62} & \multicolumn{1}{c|}{\textbf{1.38}} & \multicolumn{1}{c|}{1.41} & \multicolumn{1}{l|}{1.42} & 2.04 \\ \hline
\multicolumn{1}{|r|}{} & \multicolumn{1}{c|}{5} & \multicolumn{1}{c|}{6.6} & \multicolumn{1}{c|}{1.92} & \multicolumn{1}{c|}{1.77} & \multicolumn{1}{c|}{1.96} & \multicolumn{1}{c|}{\textbf{1.2}} & \multicolumn{1}{l|}{1.78} & 2.7 \\
\multicolumn{1}{|r|}{Phonemes} & \multicolumn{1}{c|}{10} & \multicolumn{1}{c|}{6.73} & \multicolumn{1}{c|}{1.55} & \multicolumn{1}{c|}{1.61} & \multicolumn{1}{c|}{1.6} & \multicolumn{1}{c|}{\textbf{1.15}} & \multicolumn{1}{l|}{1.62} & 2.58 \\
\multicolumn{1}{|r|}{} & \multicolumn{1}{c|}{20} & \multicolumn{1}{c|}{6.36} & \multicolumn{1}{c|}{1.33} & \multicolumn{1}{c|}{1.45} & \multicolumn{1}{c|}{1.3} & \multicolumn{1}{c|}{\textbf{1.14}} & \multicolumn{1}{l|}{1.38} & 2.28 \\ \hline
\multicolumn{1}{|r|}{} & \multicolumn{1}{c|}{5} & \multicolumn{1}{c|}{4.6} & \multicolumn{1}{c|}{0.55} & \multicolumn{1}{c|}{0.73} & \multicolumn{1}{c|}{0.58} & \multicolumn{1}{c|}{\textbf{0.39}} & \multicolumn{1}{l|}{0.98} & 1.9 \\
\multicolumn{1}{|r|}{Wilt} & \multicolumn{1}{c|}{10} & \multicolumn{1}{c|}{4.78} & \multicolumn{1}{c|}{0.43} & \multicolumn{1}{c|}{0.66} & \multicolumn{1}{c|}{0.43} & \multicolumn{1}{c|}{\textbf{0.31}} & \multicolumn{1}{l|}{0.78} & 1.81 \\
\multicolumn{1}{|r|}{} & \multicolumn{1}{c|}{20} & \multicolumn{1}{c|}{5.63} & \multicolumn{1}{c|}{0.34} & \multicolumn{1}{c|}{0.61} & \multicolumn{1}{c|}{0.36} & \multicolumn{1}{c|}{\textbf{0.3}} & \multicolumn{1}{l|}{0.57} & 1.49 \\ \hline
\multicolumn{1}{|r|}{} & \multicolumn{1}{c|}{5} & \multicolumn{1}{c|}{2.94} & \multicolumn{1}{c|}{4.06} & \multicolumn{1}{c|}{3.63} & \multicolumn{1}{c|}{3.91} & \multicolumn{1}{c|}{2.99} & \multicolumn{1}{l|}{\textbf{2.84}} & 3.01 \\
\multicolumn{1}{|r|}{Seeds} & \multicolumn{1}{c|}{10} & \multicolumn{1}{c|}{2.75} & \multicolumn{1}{c|}{3.42} & \multicolumn{1}{c|}{2.96} & \multicolumn{1}{c|}{3.14} & \multicolumn{1}{c|}{\textbf{2.25}} & \multicolumn{1}{l|}{2.69} & 2.86 \\
\multicolumn{1}{|r|}{} & \multicolumn{1}{c|}{20} & \multicolumn{1}{c|}{2.85} & \multicolumn{1}{c|}{2.53} & \multicolumn{1}{c|}{2.25} & \multicolumn{1}{c|}{2.57} & \multicolumn{1}{c|}{\textbf{1.62}} & \multicolumn{1}{l|}{2.43} & 2.49 \\ \hline
\multicolumn{1}{|r|}{} & \multicolumn{1}{c|}{5} & \multicolumn{1}{c|}{2.9} & \multicolumn{1}{c|}{3.29} & \multicolumn{1}{c|}{3.13} & \multicolumn{1}{c|}{4.1} & \multicolumn{1}{c|}{2.32} & \multicolumn{1}{l|}{\textbf{1.14}} & 1.35 \\
\multicolumn{1}{|r|}{Iris} & \multicolumn{1}{c|}{10} & \multicolumn{1}{c|}{2.6} & \multicolumn{1}{c|}{2.34} & \multicolumn{1}{c|}{2.02} & \multicolumn{1}{c|}{1.86} & \multicolumn{1}{c|}{1.15} & \multicolumn{1}{l|}{\textbf{0.91}} & 1.16 \\
\multicolumn{1}{|r|}{} & \multicolumn{1}{c|}{20} & \multicolumn{1}{c|}{2.51} & \multicolumn{1}{c|}{1.84} & \multicolumn{1}{c|}{1.48} & \multicolumn{1}{c|}{1.34} & \multicolumn{1}{c|}{\textbf{0.58}} & \multicolumn{1}{l|}{0.65} & 1 \\ \hline
\multicolumn{1}{|r|}{} & \multicolumn{1}{c|}{5} & \multicolumn{1}{c|}{4.98} & \multicolumn{1}{c|}{3.71} & \multicolumn{1}{c|}{3.56} & \multicolumn{1}{c|}{4.59} & \multicolumn{1}{c|}{3.68} & \multicolumn{1}{l|}{\textbf{3.28}} & 3.63 \\
\multicolumn{1}{|r|}{Parkinsons} & \multicolumn{1}{c|}{10} & \multicolumn{1}{c|}{5.24} & \multicolumn{1}{c|}{3.26} & \multicolumn{1}{c|}{\textbf{3.1}} & \multicolumn{1}{c|}{3.37} & \multicolumn{1}{c|}{3.11} & \multicolumn{1}{l|}{3.12} & 3.82 \\
\multicolumn{1}{|r|}{} & \multicolumn{1}{c|}{20} & \multicolumn{1}{c|}{5.1} & \multicolumn{1}{c|}{2.98} & \multicolumn{1}{c|}{3.01} & \multicolumn{1}{c|}{2.98} & \multicolumn{1}{c|}{2.96} & \multicolumn{1}{l|}{\textbf{2.91}} & 3.47 \\ \hline
\multicolumn{1}{|r|}{} & \multicolumn{1}{c|}{5} & \multicolumn{1}{c|}{2.03} & \multicolumn{1}{c|}{0.69} & \multicolumn{1}{c|}{0.78} & \multicolumn{1}{c|}{\textbf{0.22}} & \multicolumn{1}{c|}{0.29} & \multicolumn{1}{l|}{0.65} & 2.14 \\
\multicolumn{1}{|r|}{MNIST} & \multicolumn{1}{c|}{10} & \multicolumn{1}{c|}{1.86} & \multicolumn{1}{c|}{0.5} & \multicolumn{1}{c|}{0.67} & \multicolumn{1}{c|}{\textbf{0.21}} & \multicolumn{1}{c|}{0.26} & \multicolumn{1}{l|}{0.48} & 1.98 \\
\multicolumn{1}{|r|}{} & \multicolumn{1}{c|}{20} & \multicolumn{1}{c|}{1.54} & \multicolumn{1}{c|}{0.35} & \multicolumn{1}{c|}{0.53} & \multicolumn{1}{c|}{\textbf{0.2}} & \multicolumn{1}{c|}{0.22} & \multicolumn{1}{l|}{0.36} & 1.67 \\ \hline
\multicolumn{1}{|r|}{} & \multicolumn{1}{c|}{5} & \multicolumn{1}{c|}{2.3} & \multicolumn{1}{c|}{1.87} & \multicolumn{1}{c|}{1.62} & \multicolumn{1}{c|}{\textbf{1.44}} & \multicolumn{1}{c|}{1.48} & \multicolumn{1}{l|}{2.31} & 2.4 \\
\multicolumn{1}{|r|}{Fashion MNIST} & \multicolumn{1}{c|}{10} & \multicolumn{1}{c|}{2.14} & \multicolumn{1}{c|}{1.71} & \multicolumn{1}{c|}{1.52} & \multicolumn{1}{c|}{\textbf{1.41}} & \multicolumn{1}{c|}{1.46} & \multicolumn{1}{l|}{2.19} & 2.22 \\
\multicolumn{1}{|r|}{} & \multicolumn{1}{c|}{20} & \multicolumn{1}{c|}{1.92} & \multicolumn{1}{c|}{1.56} & \multicolumn{1}{c|}{1.43} & \multicolumn{1}{c|}{\textbf{1.38}} & \multicolumn{1}{c|}{1.41} & \multicolumn{1}{l|}{2.04} & 1.97 \\ \hline
\multicolumn{1}{|r|}{} & \multicolumn{1}{c|}{5} & \multicolumn{1}{c|}{5.08} & \multicolumn{1}{c|}{7.13} & \multicolumn{1}{c|}{5.85} & \multicolumn{1}{c|}{\textbf{3.76}} & \multicolumn{1}{c|}{4.27} & \multicolumn{1}{l|}{4.33} & 4.96 \\
\multicolumn{1}{|r|}{CIFAR10} & \multicolumn{1}{c|}{10} & \multicolumn{1}{c|}{4.89} & \multicolumn{1}{c|}{6.53} & \multicolumn{1}{c|}{5.3} & \multicolumn{1}{c|}{\textbf{3.91}} & \multicolumn{1}{c|}{4.4} & \multicolumn{1}{l|}{4.21} & 4.89 \\
\multicolumn{1}{|r|}{} & \multicolumn{1}{c|}{20} & \multicolumn{1}{c|}{4.77} & \multicolumn{1}{c|}{5.45} & \multicolumn{1}{c|}{4.68} & \multicolumn{1}{c|}{\textbf{3.51}} & \multicolumn{1}{c|}{3.82} & \multicolumn{1}{l|}{4.03} & 4.75 \\ \hline
\multicolumn{1}{|r|}{} & \multicolumn{1}{c|}{5} & \multicolumn{1}{c|}{10.64} & \multicolumn{1}{c|}{10.23} & \multicolumn{1}{c|}{9.88} & \multicolumn{1}{c|}{8.58} & \multicolumn{1}{c|}{8.98} & \multicolumn{1}{l|}{\textbf{7.48}} & 8.04 \\
\multicolumn{1}{|r|}{CIFAR100} & \multicolumn{1}{c|}{10} & \multicolumn{1}{c|}{10.65} & \multicolumn{1}{c|}{9.89} & \multicolumn{1}{c|}{9.38} & \multicolumn{1}{c|}{8.56} & \multicolumn{1}{c|}{9.19} & \multicolumn{1}{l|}{\textbf{7.44}} & 7.99 \\
\multicolumn{1}{|r|}{} & \multicolumn{1}{c|}{20} & \multicolumn{1}{c|}{10.66} & \multicolumn{1}{c|}{9.41} & \multicolumn{1}{c|}{8.65} & \multicolumn{1}{c|}{8.07} & \multicolumn{1}{c|}{8.81} & \multicolumn{1}{l|}{\textbf{7.33}} & 7.9 \\ \hline
\multicolumn{1}{|r|}{} & \multicolumn{1}{c|}{5} & \multicolumn{1}{c|}{3.04} & \multicolumn{1}{c|}{4.17} & \multicolumn{1}{c|}{2.16} & \multicolumn{1}{c|}{\textbf{0.89}} & \multicolumn{1}{c|}{1.35} & \multicolumn{1}{l|}{2.32} & 3.04 \\
\multicolumn{1}{|r|}{SVHN} & \multicolumn{1}{c|}{10} & \multicolumn{1}{c|}{2.98} & \multicolumn{1}{c|}{2.41} & \multicolumn{1}{c|}{2.01} & \multicolumn{1}{c|}{\textbf{0.88}} & \multicolumn{1}{c|}{1.04} & \multicolumn{1}{l|}{2.16} & 2.98 \\
\multicolumn{1}{|l|}{} & \multicolumn{1}{c|}{20} & \multicolumn{1}{c|}{2.7} & \multicolumn{1}{c|}{1.85} & \multicolumn{1}{c|}{1.54} & \multicolumn{1}{c|}{0.98} & \multicolumn{1}{c|}{\textbf{0.98}} & \multicolumn{1}{l|}{1.83} & 2.74 \\ \hline
\end{tabular}
\caption{AUC for Hard Flip corruption type.}
\end{table*}

\clearpage

\section{Additional Plots}
We provide the plots that were omitted from the main text due to space constraints.

\subsection{Plots for Experiments with Clean Auxiliary Data}
\begin{figure*}[h!]
\begin{tabular}{lll}
  \includegraphics[width=0.30\textwidth]{plots/data-phonemes_corr-Uniform_fracclean-10.png} &   \includegraphics[width=0.30\textwidth]{plots/data-phonemes_corr-Flip_fracclean-10.png}  \includegraphics[width=0.30\textwidth]{plots/data-phonemes_corr-Hard-Flip_fracclean-10.png} \\
  \includegraphics[width=0.30\textwidth]{plots/data-phonemes_corr-Uniform_fracclean-20.png} &   \includegraphics[width=0.30\textwidth]{plots/data-phonemes_corr-Flip_fracclean-20.png}  \includegraphics[width=0.30\textwidth]{plots/data-phonemes_corr-Hard-Flip_fracclean-20.png}
    \end{tabular}
    \caption{Plots for UCI Phonemes dataset at 10, 20\% clean data and all corruption types.}
\end{figure*}
 \begin{figure*}[h!]
\begin{tabular}{lll}  
 \includegraphics[width=0.30\textwidth]{plots/data-letters_corr-Uniform_fracclean-5.png} &   \includegraphics[width=0.30\textwidth]{plots/data-letters_corr-Flip_fracclean-5.png} 
 \includegraphics[width=0.30\textwidth]{plots/data-letters_corr-Hard-Flip_fracclean-5.png} \\
 \includegraphics[width=0.30\textwidth]{plots/data-letters_corr-Uniform_fracclean-10.png} &   \includegraphics[width=0.30\textwidth]{plots/data-letters_corr-Flip_fracclean-10.png} 
 \includegraphics[width=0.30\textwidth]{plots/data-letters_corr-Hard-Flip_fracclean-10.png} \\
 \includegraphics[width=0.30\textwidth]{plots/data-letters_corr-Uniform_fracclean-20.png} &   \includegraphics[width=0.30\textwidth]{plots/data-letters_corr-Flip_fracclean-20.png} 
 \includegraphics[width=0.30\textwidth]{plots/data-letters_corr-Hard-Flip_fracclean-20.png}
   \end{tabular}
   \caption{Plots for UCI Letters dataset at 5, 10, 20\% clean data and all corruption types.}
\end{figure*}
 \begin{figure*}[h!]
\begin{tabular}{lll} 
 \includegraphics[width=0.30\textwidth]{plots/data-wilt_corr-Uniform_fracclean-5.png} &   \includegraphics[width=0.30\textwidth]{plots/data-wilt_corr-Flip_fracclean-5.png} 
 \includegraphics[width=0.30\textwidth]{plots/data-wilt_corr-Hard-Flip_fracclean-5.png} \\
 \includegraphics[width=0.30\textwidth]{plots/data-wilt_corr-Uniform_fracclean-10.png} &   \includegraphics[width=0.30\textwidth]{plots/data-wilt_corr-Flip_fracclean-10.png} 
 \includegraphics[width=0.30\textwidth]{plots/data-wilt_corr-Hard-Flip_fracclean-10.png} \\
 \includegraphics[width=0.30\textwidth]{plots/data-wilt_corr-Uniform_fracclean-20.png} &   \includegraphics[width=0.30\textwidth]{plots/data-wilt_corr-Flip_fracclean-20.png} 
 \includegraphics[width=0.30\textwidth]{plots/data-wilt_corr-Hard-Flip_fracclean-20.png}
   \end{tabular}
\caption{Plots for UCI Wilt dataset at 5, 10, 20\% clean data and all corruption types.}
\end{figure*}

\begin{figure*}[h!]
\begin{tabular}{lll}  
 \includegraphics[width=0.30\textwidth]{plots/data-parkinsons_corr-Uniform_fracclean-5.png} &   \includegraphics[width=0.30\textwidth]{plots/data-parkinsons_corr-Flip_fracclean-5.png} 
 \includegraphics[width=0.30\textwidth]{plots/data-parkinsons_corr-Hard-Flip_fracclean-5.png} \\
 \includegraphics[width=0.30\textwidth]{plots/data-parkinsons_corr-Uniform_fracclean-10.png} &   \includegraphics[width=0.30\textwidth]{plots/data-parkinsons_corr-Flip_fracclean-10.png} 
 \includegraphics[width=0.30\textwidth]{plots/data-parkinsons_corr-Hard-Flip_fracclean-10.png} \\
 \includegraphics[width=0.30\textwidth]{plots/data-parkinsons_corr-Uniform_fracclean-20.png} &   \includegraphics[width=0.30\textwidth]{plots/data-parkinsons_corr-Flip_fracclean-20.png} 
 \includegraphics[width=0.30\textwidth]{plots/data-parkinsons_corr-Hard-Flip_fracclean-20.png}
   \end{tabular}
\caption{Plots for UCI Parkinsons dataset at 5, 10, 20\% clean data and all corruption types.}
\end{figure*}

 \begin{figure*}[h!]
\begin{tabular}{lll}  
 \includegraphics[width=0.30\textwidth]{plots/data-seeds_corr-Uniform_fracclean-5.png} &   \includegraphics[width=0.30\textwidth]{plots/data-seeds_corr-Flip_fracclean-5.png} 
 \includegraphics[width=0.30\textwidth]{plots/data-seeds_corr-Hard-Flip_fracclean-5.png} \\
 \includegraphics[width=0.30\textwidth]{plots/data-seeds_corr-Uniform_fracclean-10.png} &   \includegraphics[width=0.30\textwidth]{plots/data-seeds_corr-Flip_fracclean-10.png} 
 \includegraphics[width=0.30\textwidth]{plots/data-seeds_corr-Hard-Flip_fracclean-10.png} \\
 \includegraphics[width=0.30\textwidth]{plots/data-seeds_corr-Uniform_fracclean-20.png} &   \includegraphics[width=0.30\textwidth]{plots/data-seeds_corr-Flip_fracclean-20.png} 
 \includegraphics[width=0.30\textwidth]{plots/data-seeds_corr-Hard-Flip_fracclean-20.png}
   \end{tabular}
\caption{Plots for UCI Seeds dataset at 5, 10, 20\% clean data and all corruption types.}
\end{figure*}

 \begin{figure*}[h!]
\begin{tabular}{lll}  
 \includegraphics[width=0.30\textwidth]{plots/data-iris_corr-Uniform_fracclean-5.png} &   \includegraphics[width=0.30\textwidth]{plots/data-iris_corr-Flip_fracclean-5.png} 
 \includegraphics[width=0.30\textwidth]{plots/data-iris_corr-Hard-Flip_fracclean-5.png} \\
 \includegraphics[width=0.30\textwidth]{plots/data-iris_corr-Uniform_fracclean-10.png} &   \includegraphics[width=0.30\textwidth]{plots/data-iris_corr-Flip_fracclean-10.png} 
 \includegraphics[width=0.30\textwidth]{plots/data-iris_corr-Hard-Flip_fracclean-10.png} \\
 \includegraphics[width=0.30\textwidth]{plots/data-iris_corr-Uniform_fracclean-20.png} &   \includegraphics[width=0.30\textwidth]{plots/data-iris_corr-Flip_fracclean-20.png} 
 \includegraphics[width=0.30\textwidth]{plots/data-iris_corr-Hard-Flip_fracclean-20.png}
    \end{tabular}
\caption{Plots for UCI Iris dataset at 5, 10, 20\% clean data and all corruption types.}
\end{figure*}

 \begin{figure*}[h!]
\begin{tabular}{lll}  
 \includegraphics[width=0.30\textwidth]{plots/data-mnist_corr-Uniform_fracclean-5.png} &   \includegraphics[width=0.30\textwidth]{plots/data-mnist_corr-Flip_fracclean-5.png} 
 \includegraphics[width=0.30\textwidth]{plots/data-mnist_corr-Hard-Flip_fracclean-5.png} \\
 \includegraphics[width=0.30\textwidth]{plots/data-mnist_corr-Uniform_fracclean-10.png} &   \includegraphics[width=0.30\textwidth]{plots/data-mnist_corr-Flip_fracclean-10.png} 
 \includegraphics[width=0.30\textwidth]{plots/data-mnist_corr-Hard-Flip_fracclean-10.png} \\
 \includegraphics[width=0.30\textwidth]{plots/data-mnist_corr-Uniform_fracclean-20.png} &   \includegraphics[width=0.30\textwidth]{plots/data-mnist_corr-Flip_fracclean-20.png} 
 \includegraphics[width=0.30\textwidth]{plots/data-mnist_corr-Hard-Flip_fracclean-20.png}
    \end{tabular}
\caption{Plots for MNIST at 5, 10, 20\% clean data and all corruption types.}
\end{figure*}

\begin{figure*}[h!]
\begin{tabular}{lll} 
 \includegraphics[width=0.30\textwidth]{plots/data-fashion_mnist_corr-Uniform_fracclean-10.png} &   \includegraphics[width=0.30\textwidth]{plots/data-fashion_mnist_corr-Flip_fracclean-10.png} 
 \includegraphics[width=0.30\textwidth]{plots/data-fashion_mnist_corr-Hard-Flip_fracclean-10.png} \\
 \includegraphics[width=0.30\textwidth]{plots/data-fashion_mnist_corr-Uniform_fracclean-20.png} &   \includegraphics[width=0.30\textwidth]{plots/data-fashion_mnist_corr-Flip_fracclean-20.png} 
 \includegraphics[width=0.30\textwidth]{plots/data-fashion_mnist_corr-Hard-Flip_fracclean-20.png}
   \end{tabular}
\caption{Plots for Fashion MNIST at 10, 20\% clean data and all corruption types.}
\end{figure*}

 \begin{figure*}[h!]
\begin{tabular}{lll}  
 \includegraphics[width=0.30\textwidth]{plots/data-cifar10_corr-Uniform_fracclean-10.png} &   \includegraphics[width=0.30\textwidth]{plots/data-cifar10_corr-Flip_fracclean-10.png} 
 \includegraphics[width=0.30\textwidth]{plots/data-cifar10_corr-Hard-Flip_fracclean-10.png} \\
 \includegraphics[width=0.30\textwidth]{plots/data-cifar10_corr-Uniform_fracclean-20.png} &   \includegraphics[width=0.30\textwidth]{plots/data-cifar10_corr-Flip_fracclean-20.png} 
 \includegraphics[width=0.30\textwidth]{plots/data-cifar10_corr-Hard-Flip_fracclean-20.png}
 \end{tabular}
\caption{Plots for CIFAR10 at 10, 20\% clean data and all corruption types.}
\end{figure*}

\begin{figure*}[h!]
\begin{tabular}{lll}  
 \includegraphics[width=0.30\textwidth]{plots/data-cifar100_corr-Uniform_fracclean-5.png} &   \includegraphics[width=0.30\textwidth]{plots/data-cifar100_corr-Flip_fracclean-5.png} 
 \includegraphics[width=0.30\textwidth]{plots/data-cifar100_corr-Hard-Flip_fracclean-5.png} \\
 \includegraphics[width=0.30\textwidth]{plots/data-cifar100_corr-Uniform_fracclean-10.png} &   \includegraphics[width=0.30\textwidth]{plots/data-cifar100_corr-Flip_fracclean-10.png} 
 \includegraphics[width=0.30\textwidth]{plots/data-cifar100_corr-Hard-Flip_fracclean-10.png} \\
 \includegraphics[width=0.30\textwidth]{plots/data-cifar100_corr-Uniform_fracclean-20.png} &   \includegraphics[width=0.30\textwidth]{plots/data-cifar100_corr-Flip_fracclean-20.png} 
 \includegraphics[width=0.30\textwidth]{plots/data-cifar100_corr-Hard-Flip_fracclean-20.png}
    \end{tabular}
\caption{Plots for CIFAR100 at 5, 10, 20\% clean data and all corruption types.}
\end{figure*}

 \begin{figure*}[h!]
\begin{tabular}{lll}  
 \includegraphics[width=0.30\textwidth]{plots/data-svhn_corr-Uniform_fracclean-10.png} &   \includegraphics[width=0.30\textwidth]{plots/data-svhn_corr-Flip_fracclean-10.png} 
 \includegraphics[width=0.30\textwidth]{plots/data-svhn_corr-Hard-Flip_fracclean-10.png} \\
 \includegraphics[width=0.30\textwidth]{plots/data-svhn_corr-Uniform_fracclean-20.png} &   \includegraphics[width=0.30\textwidth]{plots/data-svhn_corr-Flip_fracclean-20.png} 
 \includegraphics[width=0.30\textwidth]{plots/data-svhn_corr-Hard-Flip_fracclean-20.png}
\end{tabular}
\caption{Plots for SVHN at 10, 20\% clean data and all corruption types.}
\end{figure*}

\clearpage

\subsection{Additional Plots For Experiments Without Clean Auxiliary Data}

\begin{figure*}[h!]
\begin{tabular}{lll}
  \includegraphics[width=0.30\textwidth]{plots/no_clean/data-UCI - Letters_corr-Uniform_fracclean-0.png} &   \includegraphics[width=0.30\textwidth]{plots/no_clean/data-UCI - Letters_corr-Hard-Flip_fracclean-0.png}  \includegraphics[width=0.30\textwidth]{plots/no_clean/data-UCI - Letters_corr-Flip_fracclean-0.png}
\end{tabular}
\caption{Plots for UCI Letters for all corruption types.}
\end{figure*}

\begin{figure*}[h!]
\begin{tabular}{lll}
  \includegraphics[width=0.30\textwidth]{plots/no_clean/data-UCI - Iris_corr-Uniform_fracclean-0.png} &   \includegraphics[width=0.30\textwidth]{plots/no_clean/data-UCI - Iris_corr-Hard-Flip_fracclean-0.png}  \includegraphics[width=0.30\textwidth]{plots/no_clean/data-UCI - Iris_corr-Flip_fracclean-0.png}
\end{tabular}
\caption{Plots for UCI Iris for all corruption types.}
\end{figure*}

\begin{figure*}[h!]
\begin{tabular}{lll}
  \includegraphics[width=0.30\textwidth]{plots/no_clean/data-UCI - Parkinsons_corr-Uniform_fracclean-0.png} &   \includegraphics[width=0.30\textwidth]{plots/no_clean/data-UCI - Parkinsons_corr-Hard-Flip_fracclean-0.png}  \includegraphics[width=0.30\textwidth]{plots/no_clean/data-UCI - Parkinsons_corr-Flip_fracclean-0.png}
\end{tabular}
\caption{Plots for UCI Parkinsons for all corruption types.}
\end{figure*}

\begin{figure*}[h!]
\begin{tabular}{lll}
  \includegraphics[width=0.30\textwidth]{plots/no_clean/data-UCI - Phonemes_corr-Uniform_fracclean-0.png} &   \includegraphics[width=0.30\textwidth]{plots/no_clean/data-UCI - Phonemes_corr-Hard-Flip_fracclean-0.png}  \includegraphics[width=0.30\textwidth]{plots/no_clean/data-UCI - Phonemes_corr-Flip_fracclean-0.png}
\end{tabular}
\caption{Plots for UCI Phonemes for all corruption types.}
\end{figure*}

\begin{figure*}[h!]
\begin{tabular}{lll}
  \includegraphics[width=0.30\textwidth]{plots/no_clean/data-UCI - Seeds_corr-Uniform_fracclean-0.png} &   \includegraphics[width=0.30\textwidth]{plots/no_clean/data-UCI - Seeds_corr-Hard-Flip_fracclean-0.png}  \includegraphics[width=0.30\textwidth]{plots/no_clean/data-UCI - Seeds_corr-Flip_fracclean-0.png}
\end{tabular}
\caption{Plots for UCI Seeds for all corruption types.}
\end{figure*}

\begin{figure*}[h!]
\begin{tabular}{lll}
  \includegraphics[width=0.30\textwidth]{plots/no_clean/data-UCI - Wilt_corr-Uniform_fracclean-0.png} &   \includegraphics[width=0.30\textwidth]{plots/no_clean/data-UCI - Wilt_corr-Hard-Flip_fracclean-0.png}  \includegraphics[width=0.30\textwidth]{plots/no_clean/data-UCI - Wilt_corr-Flip_fracclean-0.png}
\end{tabular}
\caption{Plots for UCI Wilt for all corruption types.}
\end{figure*}

\begin{figure*}[h!]
\begin{tabular}{lll}
  \includegraphics[width=0.30\textwidth]{plots/no_clean/data-SVHN_corr-Uniform_fracclean-0.png} &   \includegraphics[width=0.30\textwidth]{plots/no_clean/data-SVHN_corr-Hard-Flip_fracclean-0.png}  \includegraphics[width=0.30\textwidth]{plots/no_clean/data-SVHN_corr-Flip_fracclean-0.png}
\end{tabular}
\caption{Plots for SVHN for all corruption types.}
\end{figure*}

\begin{figure*}[h!]
\begin{tabular}{lll}
  \includegraphics[width=0.30\textwidth]{plots/no_clean/data-CIFAR10_corr-Uniform_fracclean-0.png} &   \includegraphics[width=0.30\textwidth]{plots/no_clean/data-CIFAR10_corr-Hard-Flip_fracclean-0.png}  \includegraphics[width=0.30\textwidth]{plots/no_clean/data-CIFAR10_corr-Flip_fracclean-0.png}
\end{tabular}
\caption{Plots for CIFAR10 for all corruption types.}
\end{figure*}

\begin{figure*}[h!]
\begin{tabular}{lll}
  \includegraphics[width=0.30\textwidth]{plots/no_clean/data-CIFAR100_corr-Uniform_fracclean-0.png} &   \includegraphics[width=0.30\textwidth]{plots/no_clean/data-CIFAR100_corr-Hard-Flip_fracclean-0.png}  \includegraphics[width=0.30\textwidth]{plots/no_clean/data-CIFAR100_corr-Flip_fracclean-0.png}
\end{tabular}
\caption{Plots for CIFAR100 for all corruption types.}
\end{figure*}
